# Supplementary material for: Constellations on the Sphere with Efficient Encoding-Decoding for Noncoherent Communications
Source: arXiv:2209.04172 source file (2022-09-09)
Supplement: Supplementary file 1 [file appendix2.tex]

\subsection{Proof of Lemma \ref{cor:integrales2}}\label{app3}
Due to space limitations, we present here a sketch of the proof, relegating the full proof to a forthcoming journal paper. We will see that the Jacobian of $\vartheta_3$ is constant and equal to $1$, which proves the lemma from the Change of Variables Theorem. In order to compute the Jacobian,  we denote the directional derivative of $\vartheta_3$ along the direction $\dot\w_i$ by  $D\vartheta_3(\w)(\dot\w_i)$. Since the function $\vartheta_3$ is not complex analytic, we need to consider its domain as a real space of dimension $2(T-1)$. Therefore, we choose orthonormal vectors $\dot\w_1,\ldots,\dot \w_{2T-4}$, which are complex orthogonal to $\w$, and complete the basis of $\mathbb C^{T-1} \equiv \mathbb{R}^{2(T-1)}$, with the two vectors $\dot \w_{2T-3}=j\w/\|\w\|$ and $\dot \w_{2T-2}=\w/\|\w\|$. 
The Jacobian of $\vartheta_3$ is the volume of the parallelepiped spanned by $\dot{\mathbf{u}}_1,\ldots,\dot{\mathbf{u}}_{2T-2}$, where $\dot{\mathbf{u}}_i$ is the projection of $D\vartheta_3(\w)(\dot\w_i)$  onto the orthogonal complement of $\left[\sqrt{1-\|\w\|^2} , \w^{\textnormal{T}}\right]^{\textnormal{T}}$. A straightforward computation yields
\begin{align*}
\dot{\mathbf{u}}_i=&\begin{bmatrix} 0 \\ \dot\w_i\end{bmatrix},\quad 1\leq i\leq 2T-4,\\
\dot{\mathbf{u}}_{2T-3}=&j\begin{bmatrix}-\|\w\|\sqrt{1-\|\w\|^2} \\ \w(1-\|\w\|^2)/\|\w\| \end{bmatrix},\\
\dot{\mathbf{u}}_{2T-2}=&\begin{bmatrix}-\|\w\|/\sqrt{1-\|\w\|^2} \\ \w/\|\w\| \end{bmatrix}.
\end{align*}
These are all mutually orthogonal vectors and hence the parallelepiped they span has volume equal to the product of their norms, which is equal to $1$.
